# Supplementary material for: Effective General-Domain Data Inclusion for the Machine Translation Task by Vanilla Transformers
Source: arXiv:2209.14073 source file (2022-09-28)
Supplement: Supplementary file 1 [file appendix.tex]

\begin{appendix}

\section{Hyperparameters}\label{sec:hyperparameters}

\begin{table}[t]
\footnotesize
	\centering\begin{tabular}{lll}
	\toprule
	Hyperparameters                    & BLINK & (T, TO, TS, TOS) \\ \midrule
	Training Batch Size                & -                                                           & 16                                                                          \\
	Validation Batch Size              & -                                                           & 16                                                                          \\
	Learning Rate                      & -                                                           & 0.00003                                                                     \\
	Number of Epochs                   & -                                                           & 5                                                                           \\
	\begin{tabular}[c]{@{}l@{}} Candidate Generation \\ Top K\end{tabular}         & 10                                                          & 10                                                                          \\
	\begin{tabular}[c]{@{}l@{}}Mention with Context \\ Max Length\end{tabular}    & 128                                                         & 128                                                                         \\
	\begin{tabular}[c]{@{}l@{}}Entity with Description \\ Max Length\end{tabular} & 128                                                         & 128                                                                         \\ \bottomrule
	\end{tabular}
	\caption{Hyperparameters configurations}
	\label{tab:hyperparameters}
\end{table}

\end{appendix}
